# Supplementary material for: Attention Lens: A Tool for Mechanistically Interpreting the Attention Head Information Retrieval Mechanism
Source: arXiv:2310.16270 source file (2023-10-25)
Supplement: Supplementary file 1 [file _appendix.tex]

\section{Outline Appendix}
\label{sec:outline}

\begin{itemize}
    \item The need for further analysis of attention heads
    \begin{itemize}
        \item Previous work covers mainly the MLP layers due to their ease of interpretability, straightforward frameworks for their understanding
        \item While we have evidence that MLP layers act as KV stores, and methods to manipulate them (ROME, GEVA, etc) we don't have a counterpart for attention heads
    \end{itemize}
    \item Attention Heads inject relevant concepts into the residual stream (often to be used in MLP lookups)
    \begin{itemize}
        \item MLP layers are KV stores, and downstream from attention heads. There is a clear relationship between the output of attn and the output of MLPs
        \item Mathematically attention head outputs combine to construct the key for MLP layers (via ROME, Geva - https://aclanthology.org/2021.emnlp-main.446/)
        \item Empirical evidence (ours) shows that attn heads inject concepts relevant to the final output, guide the iterative updates throughout each layer
        \item Furthermore, we (and others [Nanda somewhere]) can identify specialized functions for attention heads
    \end{itemize}

    \item Attention Lens can shed light on the information retrieval mechanism of transformers (and how/why they go awry in their predictions)
    
    \begin{itemize}
        \item Relation to logit lens and tuned lens
        \item Evidence for a separate/differentiated representation space in attention heads (? maybe not true - we'll see)
        \item Attention lens design and justification
        \item Attention Lens Results, characterization
    \end{itemize}

    \item Intervening on networks with the attention lens
    \begin{itemize}
        \item overview of methodology
        \item the importance of input/output representation
        \item encoding information in attention heads using the attention lens
        \item results, comparison to activation steering
        \item applications
    \end{itemize}

\end{itemize}
